# Supplementary material for: Proposal to improve Ni-based superconductors via enhanced charge transfer
Source: arXiv:2101.11169 source file (2022-12-14)
Supplement: Supplementary file 1 [file Supplementary.pdf]

# Supplementary materials: A proposal of improving Ni-based superconductors

Zi-Jian Lang, Ruoshi Jiang, and Wei Ku

## Details in density functional calculation

The phonon spectrum calculation uses density-functional perturbation theory (DFPT) method [S1] with  $4 \times 4 \times 5$   $\mathbf{k}$  mesh in self-consistent calculation and  $4 \times 4 \times 5$   $\mathbf{q}$  mesh implemented in ABINIT [S2]. The  $f$  orbitals of Nd are treated as frozen core. We use PBEsol pseudopotential [S3]. The calculation of band structures uses LDA+ $U$  via linearized augmented plane wave (LAPW) method [S4, S5] implemented in WIEN2k [S6] with on-site repulsion parameters,  $U - J = 0.6 - 0.06 = U_{eff} = 0.54$  Ry for Cu/Ni  $d$  orbitals,  $U_{eff} = 0.2, 0.6$  Ry for Nd  $d$  and  $f$  orbitals. The lattice parameters are  $a = b = 3.86\text{\AA}$ ,  $c = 3.20\text{\AA}$  for CaCuO<sub>2</sub> [S7], and  $a = b = 3.92\text{\AA}$ ,  $c = 3.37\text{\AA}$  for NdNiO<sub>2</sub> [S8], both with P4/mmm space group. And the antiferromagnetic (AFM) ordered phase use  $\sqrt{2} \times \sqrt{2} \times 2$  supercell with  $G$ -type spin configuration.

## 10 eV-scale effective interacting Hamiltonian

To get the low-energy effective Hamiltonian in Eq.(1), we first need the high-energy ( $\sim 10\text{eV}$ -scale) 4-orbital effective interacting Hamiltonian of holes including  $d_{x^2-y^2}, d_{3z^2-r^2}$  and two  $p_{||}$  orbitals [S9]:

$$H^{eff} = \sum_{i,m,v} \epsilon_{im} n_{imv} + \sum_{i,i',m,m',v} t_{ii'mm'} c_{imv}^\dagger c_{i'm'v} + \sum_{\langle j,i \rangle m} J_m \mathbf{S}_j^F \cdot \mathbf{S}_{im} + \sum_{i,d,d',v} U_{dd'} n_{idv} n_{id'v} + \sum_{i,d,d' \neq d,v} (U_{dd'} - J_{dd'}) n_{idv} n_{id'v}, \quad (S1)$$

where  $c_{imv}^\dagger$  and  $n_{imv} \equiv c_{imv}^\dagger c_{imv}$  denote the creation and number operator of holes of spin  $v$  in orbital  $m$  of site  $i$  that experience kinetic hopping  $t_{ii'mm'}$  and orbital energy  $\epsilon_{im}$ .  $\mathbf{S}_{im} = \sum_{v,v'} c_{imv}^\dagger \boldsymbol{\sigma}_{v,v'} c_{imv}$  denotes the orbital-dependent spin operator and  $\boldsymbol{\sigma}_{v,v'}$  is the vector of Pauli matrices. Since the orbital dependent coupling to the 3/2 spin  $\mathbf{S}^F$  of nearest Nd- $f$  orbitals at location  $j$  is negligibly weak ( $< 50\text{meV}$ ) [S9], we did not list the value of  $J_m$  here.

We then require the Hartree-Fock approximation of our  $H^{eff}$  to reproduce the LDA+ $U$  band structure (or equivalently the Kohn-Sham Hamiltonian) within the subspace of these four active orbitals to obtain a set of realistic parameters in  $H^{eff}$  [S10]. This mapping makes sense because the LDA+ $U$  approximation employs a similar treatment of the intra-atomic many-body interactions. Specifically, we obtain  $t_{ii'}$  from the LDA+ $U$  Kohn-Sham Hamiltonian,  $H^{LDA+U}$ , represented in atomic Wannier orbitals [S11]. We then approximate  $U_{dd'}$  and  $J_{dd'}$  via a Slater integral [S4, S12] with  $U_{eff}$  and  $J_{eff}$ , which are treated as the only fitting parameters. With  $U_{dd'}$ ,  $J_{dd'}$  and  $J_m$  fixed,  $\epsilon_{im}$  can be obtained by subtracting the mean-field of Hartree-Fock and  $J_m$  from the above  $H^{LDA+U}$  and requires both spin channels to have the same value [S10]. Here,  $U^{eff} = 8.3, 7.4$  and  $7.4$  eV,  $J^{eff} = 1.1, 0.95$  and  $1.2$  eV can

well reproduce the LDA+ $U$  results of CaCuO<sub>2</sub>, NdNiS<sub>2</sub> and NdNiO<sub>2</sub> under ferromagnetic(FM) and antiferromagnetic order as shown in Figure S1. We set the on-site repulsion of oxygen atoms  $U_{pp} = 4\text{eV}$  [S13] in our exact diagonalization process.

Table S1- S3 show the local on-site and kinetic energy in  $H^{eff}$  for these three materials respectively.

## Additional results about Nd electron carriers

Our calculation shows that the coupling of orbital space hosting electron and hole carriers is very weak ( $\sim 0.1\text{eV}$ ) compared with their energy separation ( $\sim 5\text{eV}$ ). There is no direct or indirect coupling between Ni  $d_{x^2-y^2}$  and Nd  $d_{3z^2-r^2}$  or  $d_{xy}$  orbitals due to the symmetry. This weak  $\sim 0.1\text{eV}$  coupling only exists between Ni  $d_{3z^2-r^2}$  and Nd  $d_{3z^2-r^2}$  or  $d_{xy}$  orbitals.

TABLE S1. Local on-site and kinetic energy in  $H^{eff}$  of CaCuO<sub>2</sub> for Cu- $d_{x^2-y^2}$ ,  $d_{3z^2-r^2}$ , and two O- $p_{||}$  orbitals pointing toward Cu from the two O sites next to Cu.

| $H^{LDA+U}$ (eV) | $d_{x^2-y^2}$ | $d_{3z^2-r^2}$ | $p_{  }(p_x)$ | $p_{  }(p_y)$ |
|------------------|---------------|----------------|---------------|---------------|
| $d_{x^2-y^2}$    | 0.51          | 0              | -1.29         | 1.29          |
| $d_{3z^2-r^2}$   | 0             | 0.67           | 0.40          | 0.40          |
| $p_{  }(p_x)$    | -1.29         | 0.40           | 4.23          | 0.65          |
| $p_{  }(p_y)$    | 1.29          | 0.40           | 0.65          | 4.23          |

TABLE S2. Local on-site and kinetic energy in  $H^{eff}$  of NdNiS<sub>2</sub> for Ni- $d_{x^2-y^2}$ ,  $d_{3z^2-r^2}$ , and two S- $p_{||}$  orbitals pointing toward Ni from the two S sites next to Ni.

| $H^{LDA+U}$ (eV) | $d_{x^2-y^2}$ | $d_{3z^2-r^2}$ | $p_{  }(p_x)$ | $p_{  }(p_y)$ |
|------------------|---------------|----------------|---------------|---------------|
| $d_{x^2-y^2}$    | -1.75         | 0              | 1.17          | -1.17         |
| $d_{3z^2-r^2}$   | 0             | -2.26          | -0.42         | -0.42         |
| $p_{  }(p_x)$    | 1.17          | -0.42          | 3.97          | 0.84          |
| $p_{  }(p_y)$    | -1.17         | -0.42          | 0.84          | 3.97          |

TABLE S3. Local on-site and kinetic energy in  $H^{eff}$  of NdNiO<sub>2</sub> for Ni- $d_{x^2-y^2}$ ,  $d_{3z^2-r^2}$ , and two O- $p_{||}$  orbitals pointing toward Ni from the two O sites next to Ni.

| $H^{LDA+U}$ (eV) | $d_{x^2-y^2}$ | $d_{3z^2-r^2}$ | $p_{  }(p_x)$ | $p_{  }(p_y)$ |
|------------------|---------------|----------------|---------------|---------------|
| $d_{x^2-y^2}$    | -3.88         | 0              | -1.37         | 1.37          |
| $d_{3z^2-r^2}$   | 0             | -3.39          | 0.40          | 0.40          |
| $p_{  }(p_x)$    | -1.37         | 0.40           | 5.06          | 0.65          |
| $p_{  }(p_y)$    | 1.37          | 0.40           | 0.65          | 5.06          |

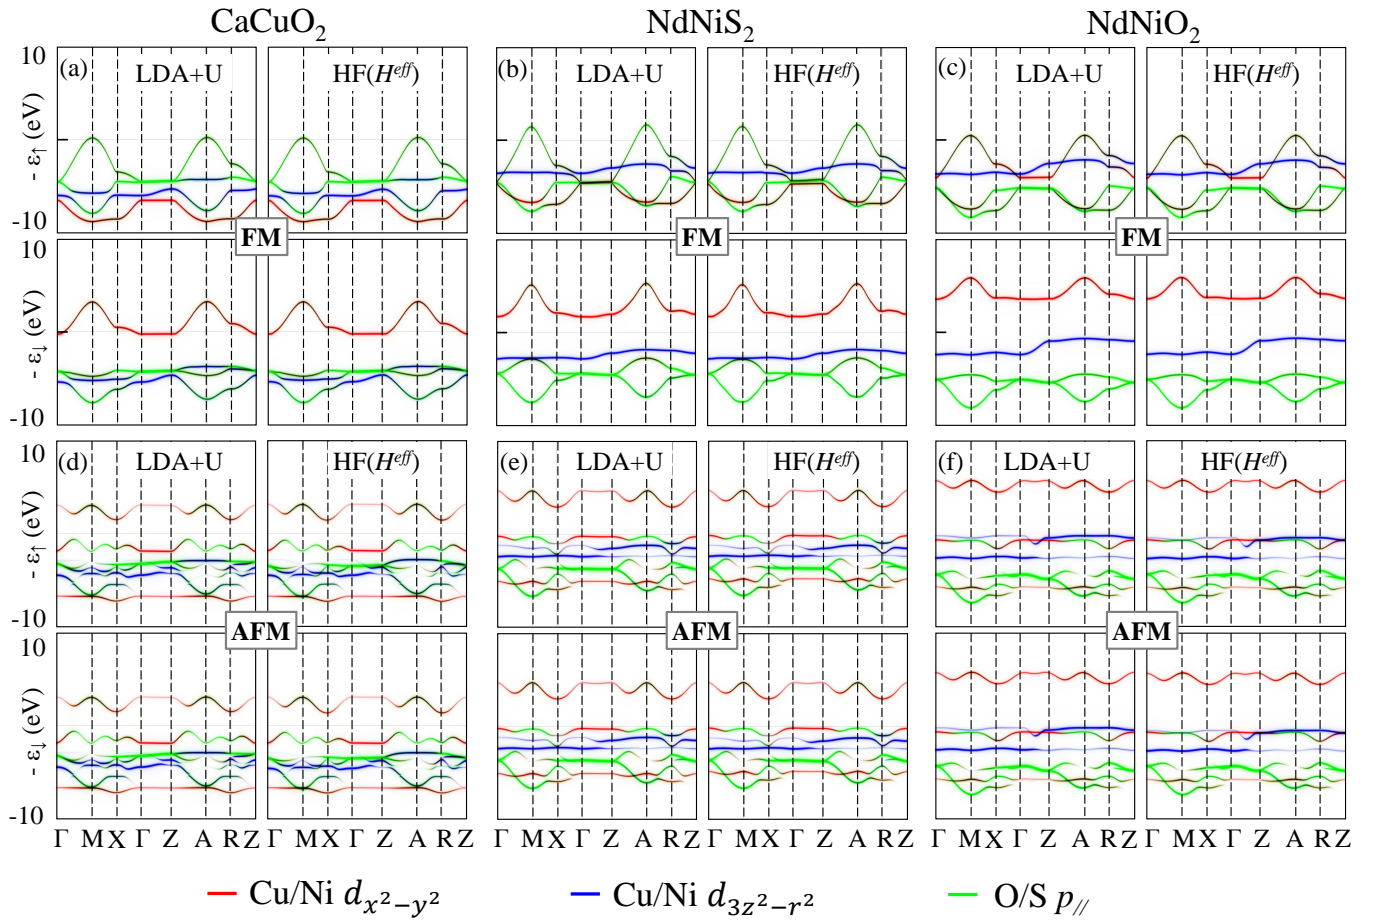

FIG. S1. Comparison of the Hartree-Fock band structures of the four-orbital model and those of LDA+ $U$  ones within the same Cu/Ni (red)  $d_{x^2-y^2}$ , (blue)  $d_{3z^2-r^2}$  and (green) O/S  $p_{\parallel}$  subspace, under FM [(a)(b)(c)] and AFM [(d)(e)(f)] order for  $\text{CaCuO}_2$ ,  $\text{NdNiS}_2$  and  $\text{NdNiO}_2$ .

- 
- [S1] S. Baroni, S. de Gironcoli, A. Dal Corso, and P. Giannozzi, *Rev. Mod. Phys.* **73**, 515 (2001).
- [S2] X. Gonze, B. Amadon, G. Antonius, F. Arnardi, L. Baguet, J.-M. Beuken, J. Bieder, F. Bottin, J. Bouchet, E. Bousquet, N. Brouwer, F. Bruneval, G. Brunin, T. Cavignac, J.-B. Charraud, W. Chen, M. Côté, S. Cottenier, J. Denier, G. Geneste, P. Ghosez, M. Giantomassi, Y. Gillet, O. Gingras, D. R. Hamann, G. Hautier, X. He, N. Helbig, N. Holzwarth, Y. Jia, F. Jollet, W. Lafargue-Dit-Hauret, K. Lejaeghere, M. A. Marques, A. Martin, C. Martins, H. P. Miranda, F. Naccarato, K. Persson, G. Petretto, V. Planes, Y. Pouillon, S. Prokhorenko, F. Ricci, G.-M. Rignanese, A. H. Romero, M. M. Schmitt, M. Torrent, M. J. van Setten, B. Van Troeye, M. J. Verstraete, G. Zérah, and J. W. Zwanziger, *Computer Physics Communications* **248**, 107042 (2020).
- [S3] D. R. Hamann, *Phys. Rev. B* **88**, 085117 (2013).
- [S4] A. I. Liechtenstein, V. I. Anisimov, and J. Zaanen, *Phys. Rev. B* **52**, R5467 (1995).
- [S5] V. I. Anisimov, I. V. Solovyev, M. A. Korotin, M. T. Czyżyk, and G. A. Sawatzky, *Phys. Rev. B* **48**, 16929 (1993).
- [S6] P. Blaha, K. Schwarz, F. Tran, R. Laskowski, G. K. H. Madsen, and L. D. Marks, *The Journal of Chemical Physics* **152**, 074101 (2020).
- [S7] E. Kopnin, H. Schwer, J. Jun, G. Meijer, R. Molinski, K. Conder, and J. Karpinski, *Physica C: Superconductivity* **282-287**, 483 (1997), proceedings of the International Conference on Materials and Mechanisms of Superconductivity High Temperature Superconductors V Part II.
- [S8] D. Li, K. Lee, B. Y. Wang, M. Osada, S. Crossley, H. R. Lee, Y. Cui, Y. Hikita, and H. Y. Hwang, *Nature* **572**, 624 (2019).
- [S9] Z.-J. Lang, R. Jiang, and W. Ku, arXiv e-prints, arXiv:2005.00022 (2020), arXiv:2005.00022 [cond-mat.supr-con].
- [S10] W.-G. Yin, D. Volja, and W. Ku, *Phys. Rev. Lett.* **96**, 116405 (2006).
- [S11] W. Ku, H. Rosner, W. E. Pickett, and R. T. Scalettar, *Phys. Rev. Lett.* **89**, 167204 (2002).
- [S12] J. Slater, *Quantum Theory of Molecules and Solids* (Mcgram-Hill, New York, 1974).
- [S13] M. Ogata and H. Fukuyama, *Reports on Progress in Physics* **71**, 036501 (2008).
